# Supplementary material for: Enhanced Signal Recovery via Sparsity Inducing Image Priors
Source: arXiv:1805.04828 source file (2018-05-13)
Supplement: Supplementary file 2 [file Appendix-B.tex]

\Appendix{DOI Afterthoughts}

\section{Introduction}
When in the Course of human events, it becomes necessary for one people  to dissolve the political bands which have connected them with another,  and to assume among the powers of the earth, the separate and equal station  to which the Laws of Nature and of Nature's God entitle them, a decent respect to the opinions of mankind requires that they should declare  the causes which impel them to the separation.

\section{More Declaration}

We hold these truths to be self-evident, that all men are created equal,  that they are endowed by their Creator with certain unalienable Rights,  that among these are Life, Liberty and the pursuit of Happiness. --That to secure these  rights, Governments are instituted among Men, deriving their just powers  from the consent of the governed, --That whenever any Form of Government  becomes destructive of these ends, it is the Right of the People to alter  or to abolish it, and to institute new Government, laying its foundation on  such principles and organizing its powers in such form, as to them shall  seem most likely to effect their Safety and Happiness. Prudence, indeed, will dictate that Governments long established should not  be changed for light and transient causes; and accordingly all experience  hath shewn, that mankind are more disposed to suffer, while evils are  sufferable, than to right themselves by abolishing the forms to which they  are accustomed. But when a long train of abuses and usurpations, pursuing invariably the same  Object evinces a design to reduce them under absolute Despotism, it is their  right, it is their duty, to throw off such Government, and to provide new Guards for their future security. --Such has been the patient sufferance of these Colonies; and such is now the  necessity which constrains them to alter their former Systems of Government.  The history of the present King of Great Britain [George III] is a history  of repeated injuries and usurpations, all having in direct object the  establishment of an absolute Tyranny over these States. To prove this, let Facts be submitted to a candid world.
