# Supplementary material for: Enhanced Signal Recovery via Sparsity Inducing Image Priors
Source: arXiv:1805.04828 source file (2018-05-13)
Supplement: Supplementary file 5 [file Dedication.tex]

To my beloved parents
