# Supplementary material for: Enhanced Signal Recovery via Sparsity Inducing Image Priors
Source: arXiv:1805.04828 source file (2018-05-13)
Supplement: Supplementary file 6 [file ListOfSymbols.tex]

% Place the list of symbols below.
\begin{eqlist}[\labelsep 1em]

\item[$\alpha$]
The first greek letter, p.~\pageref{}

\item[$\alpha$]
The first greek letter, p.~\pageref{}

\item[$\alpha$]
The first greek letter, but we should really add some more text, though we need it to go on two lines, p.~\pageref{}

\item[$\alpha$]
The first greek letter, p.~\pageref{}

\item[$\alpha$]
The first greek letter, p.~\pageref{}

\item[$\alpha$]
The first greek letter, p.~\pageref{}

\item[$\alpha$]
The first greek letter, p.~\pageref{}

\item[$\alpha$]
The first greek letter, p.~\pageref{}

\end{eqlist}
